# Supplementary material for: Universal Semi-supervised Model Adaptation via Collaborative Consistency Training
Source: arXiv:2307.03449 source file (2023-11-03)
Supplement: Supplementary file 1 [file supp.tex]

\begin{table*}[t]
    \centering
    \caption{H-score on \textit{Domainnet} under the settings of 3-shot using ResNet34 as the backbone.}
    \setlength\tabcolsep{3pt}
    \scalebox{1}{
        \begin{tabular}{l|ccccccc}
        \toprule
        \textbf{Method}
        &  R $\rightarrow$ C
        &  P $\rightarrow$ C
        &  C $\rightarrow$ S
        &  R $\rightarrow$ P
        &  S $\rightarrow$ P
        &  R $\rightarrow$ S
        & \textbf{Mean} \\  
        \midrule
        CE       & 50.8 & 53   & 47.1 & 50.3 & 53.5 & 43.6 & 49.7 \\
        ENT      & 45.9 & 44.3 & 36.0 & 36.8 & 43.0 & 36.3 & 40.4 \\
        MixMatch & 48.0 & 50.5 & 44.4 & 50.1 & 50.2 & 44.2 & 47.9 \\
        FixMatch & 52.5 & 48.2 & 49.8 & 52.8 & 48.6 & 43.0 & 49.2 \\
        UMA      & 42.7 & 46.2 & 41.7 & 42.9 & 40.4 & 40.2 & 42.3 \\
        MME      & 56.7 & 58.9 & 45.0 & 49.9 & 52.7 & 42.8 & 51.0 \\
        CDAC     & 59.0 & 59.2 & 50.8 & 62.3 & 62.3 & 51.9 & 57.6 \\
        SSHT     & 64.1 & 66.8 & 54.2 & 59.0 & 65.6 & 47.1 & 59.5 \\
        SHOT++   & 55.6 & 59.4 & 51.0 & 56.1 & 56.7 & 45.4 & 54.0 \\
        CCT      & \textbf{69.9} & \textbf{69.0} & \textbf{58.6} & \textbf{66.7} & \textbf{67.4} & \textbf{56.2} & \textbf{64.6} \\
        \bottomrule
        \end{tabular}
    }
    \label{table:3shot_domainnet}
\end{table*}
\begin{table*}[t]
    \centering
    \caption{ H-score on \textit{Office-Home} under the settings of 3-shot using ResNet34 as the backbone.}
    \setlength\tabcolsep{2.1pt}
    \scalebox{1}{
        \begin{tabular}{l|ccccccccccccc}
        \toprule
        \textbf{Method}
        & \small A $\rightarrow$ C
        & \small A $\rightarrow$ P
        & \small A $\rightarrow$ R
        & \small C $\rightarrow$ A
        & \small C $\rightarrow$ P
        & \small C $\rightarrow$ R
        & \small P $\rightarrow$ A
        & \small P $\rightarrow$ C
        & \small P $\rightarrow$ R
        & \small R $\rightarrow$ A
        & \small R $\rightarrow$ C
        & \small R $\rightarrow$ P
        & \textbf{Mean} \\  
        \midrule
        CE       & 51.8 & 73.9 & 69.9 & 49.9 & 70.7 & 65.6 & 57.8 & 51.1 & 68.9 & 55.7 & 54.0 & 74.6 & 62.0 \\
        ENT      & 53.2 & 76.4 & 71.7 & 46.3 & 74.9 & 66.1 & 54.6 & 46.5 & 69.4 & 57.3 & 54.8 & 77.2 & 62.4 \\
        MixMatch & 51.3 & 77.6 & 73.3 & 51.8 & 76.4 & 69.7 & 56.8 & 51.1 & 72.2 & 58.3 & 53.4 & 78.5 & 64.2 \\
        FixMatch & 50.6 & 76.2 & 67.5 & 39.9 & 76.6 & 66.9 & 53.9 & 56.7 & 67.4 & 47.1 & 51.8 & 75.4 & 60.8 \\
        UMA     & 54.6 & 76.3 & 71.3 & 52.1 & 73.7 & 63.3 & 57.2 & 52.5 & 68.8 & 54.0 & 56.4 & 76.2 & 63.0 \\
        MME      & 55.6 & 77.1 & 72.3 & 55.2 & 75.3 & 68.8 & 60.0 & 53.6 & 72.5 & 61.4 & 57.8 & 77.3 & 65.6 \\
        CDAC     & 55.7 & 76.3 & 72.0 & 54.0 & 75.4 & 68.9 & 54.5 & 58.8 & 72.3 & 60.6 & 57.1 & 76.9 & 65.2 \\
        SSHT     & 55.0 & 73.0 & 69.9 & 56.0 & 72.3 & 67.0 & 51.4 & 53.9 & 68.6 & 58.0 & 59.1 & 74.0 & 63.2 \\
        SHOT++   & 54.9 & 80.3 & 74.2 & 53.3 & 73.9 & 70.8 & 55.9 & 52.3 & 76.9 & 50.2 & 52.7 & 79.3 & 64.6 \\
        CCT     & \textbf{57.8} & \textbf{80.6} & \textbf{77.3} & \textbf{61.0} & \textbf{79.4} & \textbf{76.9} & \textbf{62.6} & \textbf{57.8} & \textbf{77.1} & \textbf{63.4} & \textbf{59.2} & \textbf{80.2} & \textbf{69.4} \\
        \bottomrule
        \end{tabular}
    }
    \label{table:3shot_office_home}
\end{table*}

\section{Additional Results}
\subsection{Results on 3-shot Setting}
In addition to the results of the 5-shot and 10-shot settings presented in the main paper, we further show the results of \textit{Domainnet} and \textit{Office-Home} in the 3-shot setting, as shown in Table~\ref{table:3shot_domainnet} and Table~\ref{table:3shot_office_home} respectively. Similar to those in the 5-shot and 10-shot settings, our proposed CCT outperforms all the compared methods in the 3-shot setting. It is worth noting that our CCT surpasses all compared methods for all domain pairs, and the performance gaps are even larger than those of 5-shot and 10-shot settings. 

\input{latex/sup_misc/ssma}
\begin{table}[t]
    \centering
    % \vspace{-2mm}
    \caption{Results of different pseudo label generation strategies for sample-wise consistency on \textit{Domainnet}}
    \setlength\tabcolsep{10pt}
    \scalebox{0.8}{
        \begin{tabular}{l|cc}
        \toprule
        \textbf{Consistency Loss}
         & R $\rightarrow$ C
        & C $\rightarrow$ S \\
        \midrule
        Ensemble & 75.3 & 65.6 \\
        Weighted ensemble & 75.4 & 65.6 \\
        Sample-wise & \textbf{77.7} & \textbf{66.8}   \\
        \bottomrule
        \end{tabular}
    }
    \label{table:pl}
\end{table}
\begin{table}[t]
    \centering
    \caption{H-score of R $\rightarrow$ P and S $\rightarrow$ P on \textit{Domainnet} 5 settings.}
    \setlength\tabcolsep{10pt}
    \scalebox{0.8}{
        \begin{tabular}{l|cc}
        \toprule
         \textbf{Method}
        &  { R $\rightarrow$ P} 
        &  { S $\rightarrow$ P} \\
        \midrule
        RotPred & 71.8 & 73.9 \\
        SCL+SimCLR & \textbf{75.5} & \textbf{75.3}  \\
        \bottomrule
        \end{tabular}
    }
    \label{table:ssl}
\end{table}
\begin{table}[t]
    \centering
    \caption{H-score on the \textit{Domainnet} 5-shot setting.}
    \setlength\tabcolsep{2.4pt}
    \scalebox{0.8}{
        \begin{tabular}{l|ccccccc}
        \toprule
        \small \textbf{Method}
        &  \small \rotatebox[origin=c]{0}{R $\rightarrow$ C}
        &  \small \rotatebox[origin=c]{0}{P $\rightarrow$ C}
        &  \small \rotatebox[origin=c]{0}{C $\rightarrow$ S}
        &  \small \rotatebox[origin=c]{0}{R $\rightarrow$ P}
        &  \small \rotatebox[origin=c]{0}{S $\rightarrow$ P}
        &  \small \rotatebox[origin=c]{0}{R $\rightarrow$ S}
        & \small \textbf{Mean} \\  
        \midrule
        $F(\cdot|\theta_s)$ & 77.7 & 77.4 & 66.8 & 75.5 & 75.3 & 66.9 & \textbf{73.3} \\
        $F(\cdot|\theta_t)$ & 77.9 & 77.4 & 66.7 & 75.5 & 75.1 & 66.8 & 73.2 \\
        \bottomrule
        \end{tabular}
    }
    \label{table:result_F}
\end{table}

\subsection{Results on SSMA Benchmark}
In addition to Universal Semi-supervised Model Adaptation~(USMA), we also implement CCT on Semi-supervised Model Adaptation~(SSMA) benchmark. Following~\cite{shotplus}, we conduct experiments on \textit{Office-Home} 1-shot setting using VGG16 as the backbone. The mean accuracy over 12 domain pairs is shown in Table~\ref{table:ssma}. It can be observe that CCT outperforms the current SOTA: SHOT++~\cite{shotplus}, which further demonstrates the versatility of CCT.

\begin{table*}[t]
    \centering
    \caption{ Accuracy of Common~($a_{\mathcal{C}}$) and Private~($a_{\mathcal{P}}$) set on the \textit{DomainNet} 5-shot setting using ResNet34 as the backbone.}
    \setlength\tabcolsep{8pt}
    \scalebox{0.8}{
        \begin{tabular}{l|cccccccccccccc}
        \toprule
        & \multicolumn{2}{c}{R $\rightarrow$ C} 
        & \multicolumn{2}{c}{P $\rightarrow$ C} 
        & \multicolumn{2}{c}{C $\rightarrow$ S}
        & \multicolumn{2}{c}{R $\rightarrow$ P} 
        & \multicolumn{2}{c}{S $\rightarrow$ P}
        & \multicolumn{2}{c}{R $\rightarrow$ S} 
        % & \multicolumn{2}{c|}{P $\rightarrow$ R}
        & \multicolumn{2}{c}{\textbf{Mean}} \\  
        \textbf{Method}
        & \small $a_{\mathcal{C}}$ & \small $a_{\mathcal{P}}$
        & \small $a_{\mathcal{C}}$ & \small $a_{\mathcal{P}}$
        & \small $a_{\mathcal{C}}$ & \small $a_{\mathcal{P}}$
        & \small $a_{\mathcal{C}}$ & \small $a_{\mathcal{P}}$
        & \small $a_{\mathcal{C}}$ & \small $a_{\mathcal{P}}$
        & \small $a_{\mathcal{C}}$ & \small $a_{\mathcal{P}}$
        % & \small 1-shot & \small Private
        & \small \textbf{$a_{\mathcal{C}}$} & \small \textbf{$a_{\mathcal{P}}$}\\
        \midrule
       CE       & 73.6 & 47.9 & 72.2 & 47.4 & 65.5 & 46.8 & 67.3 & 50.4 & 67.3 & 51.4 & 65.0 & 41.4 & 68.5 & 47.6 \\
        MME      & 74.8 & 59.8 & 73.7 & 56.7 & 62.4 & 49.5 & 63.1 & 61.6 & 65.8 & 61.9 & 62.4 & 43.4 & 67.0 & 55.5 \\
        FixMatch & 82.2 & 58.9 & 81.8 & 55.9 & 72.7 & 52.8 & 71.5 & 65.7 & 73.9 & 63.4 & 73.1 & 57.1 & 75.9 & 59.0 \\
        CCT      & \textbf{83.0} & \textbf{73.1} & \textbf{81.6} & \textbf{73.6} & \textbf{74.1} & \textbf{60.8} & \textbf{77.3} & \textbf{73.8} & \textbf{75.8} & \textbf{74.7} & \textbf{75.1} & \textbf{60.2} & \textbf{77.8} & \textbf{69.4} \\
        \bottomrule
        \end{tabular}
    }
    \label{table:Common_Private_acc}
\end{table*}
\begin{table}[t]
    \centering
    \caption{(a) Average H-score w.r.t. loss weight $\lambda_1$ on the  \textit{Office-Home} 5-shot setting. Note that $\lambda_2$ is fixed to 0.5. (b) Average H-score w.r.t. loss weight $\lambda_2$ on the  \textit{Office-Home} 5-shot setting. Note that $\lambda_1$ is fixed to 1.}
    \begin{minipage}{0.49\textwidth}
            \centering
            \setlength\tabcolsep{5.5pt}
            \scalebox{0.8}{
                \begin{tabular}{l|cccc}
                \toprule
                $\lambda_1$ & 0 & 0.5 &  1 &  1.5 \\
                \midrule
                H-score & 72.3 & 73.5 & 73.5 & 72.8 \\
                \bottomrule
                \end{tabular}
            } \\ \vspace{1mm} (a) \vspace{1mm}
    \end{minipage}
    \begin{minipage}{.49\textwidth}
            \centering
            \setlength\tabcolsep{5.5pt}
            \scalebox{0.8}{
                \begin{tabular}{l|cccc}
                \toprule
                $\lambda_2$ & 0 & 0.5 &  1 &  1.5 \\
                \midrule
                H-score & 70.5 & 73.5 & 73.3 & 72.6 \\
                \bottomrule
                \end{tabular}
            }\\ \vspace{1mm}(b)
        % \end{table}
    \end{minipage}%
    \label{tab:lambda}
    \vspace{-2mm}
\end{table}

\section{Additional Analysis}
\subsection{Pseudo Label Generation Strategy}
We empirically validate multiple pseudo label generation strategies, \eg \textit{ensemble} and \textit{weighted ensemble}, where \textit{ensemble} refers to the strategy where pseudo labels are generated by thresholding $[F(x^{\prime}|\theta_s) + F(x^{\prime}|\theta_t)] / 2$, and \textit{weighted ensemble} refers to the strategy of thresholding $[wF(x^{\prime}|\theta_s) + (1 - w)F(x^{\prime}|\theta_t)]$, where $w \in [0, 1]$ is computed by the entropy of the two networks. As Table~\ref{table:pl} shows, our $L_{sample}$ is more effective.

\subsection{Justification of Our $F(\cdot|\theta_t)$ Pre-training Method}
To justify our choice of the pre-training method, SCL~\cite{khosla2020scl} + SimCLR~\cite{chen2020simclr}, for $F(\cdot|\theta_t)$, we compare it with rotation prediction~\cite{gidaris2018unsupervised} on \textit{Real} $\rightarrow$ \textit{Painting} and \textit{Sketch} $\rightarrow$ \textit{Painting} of \textit{Domainnet}. As shown in Table~\ref{table:ssl}, our SCL~\cite{khosla2020scl} + SimCLR~\cite{chen2020simclr} yields better results than rotation prediction~\cite{gidaris2018unsupervised}.

\subsection{Justification of Choice between $F(\cdot|\theta_s)$ and $F(\cdot|\theta_t)$}
As mentioned in the main paper, the performance of $F(\cdot|\theta_s)$ and $F(\cdot|\theta_t)$ will converge to the same point after training and thus we simply choose $F(\cdot|\theta_s)$ as the final model. To support our choice, we show the H-score of $F(\cdot|\theta_s)$ and $F(\cdot|\theta_t)$ on \textit{Domainnet} in Table~\ref{table:result_F}. It can be observed that the performance of $F(\cdot|\theta_s)$ and $F(\cdot|\theta_t)$ are very close, and $F(\cdot|\theta_s)$ performs slightly better, which justifies our choice.

\subsection{Accuracy of Common-Private Set Samples}
In addition to H-score, we also report the accuracy of common and private set samples on \textit{Domainnet}. As Table~\ref{table:Common_Private_acc} shows, the accuracy of private set significantly outperforms all compared methods. It is worth noting that i) the performance gap between common set accuracy of FixMatch and CCT is relatively small, ii) while for the private set accuracy, the gap is significant larger, which implies that the CCT can effectively improve the performance of $F(\cdot|\theta_s)$ on private set.

\subsection{Analysis of Hyper-parameters}
The proposed CCT has three hyper-parameters, \ie the threshold $\tau$, the loss weight of sample-wise consistency $\lambda_1$, and the loss weight of class-wise consistency $\lambda_2$. In this section, we study how $\lambda_1$ and $\lambda_2$ influence the performance since $\tau$ has been studied in the main paper. We conduct the experiments on \textit{Office-Home}. As Table~\ref{tab:lambda} shows, we achieve the best performance when $\lambda_1 = 1$ and $\lambda_2 = 0.5$. It can be observed that when $\lambda_2 = 0$, \ie without sample-wise consistency, the performance is much lower, which demonstrates the efficacy of our sample-wise consistency. Furthermore, it can be observed that the model is not sensitive w.r.t $\lambda_1$ and $\lambda_2$.

\subsection{Analysis of Performance Stability}
\begin{table}[t]
    \centering
    \caption{Mean and standard deviation of H-score over five runs on \textit{Domainnet} on the 5-shot setting. Note that \textbf{Avg} denotes the Mean and standard deviation of the mean H-score over five runs.}
    \setlength\tabcolsep{2.5pt}
    \scalebox{1}{
        \begin{tabular}{l|ccccccc}
        \toprule
        \small \textbf{Method}
        &  \small \rotatebox[origin=c]{0}{R $\rightarrow$ C}
        &  \small \rotatebox[origin=c]{0}{P $\rightarrow$ C}
        &  \small \rotatebox[origin=c]{0}{C $\rightarrow$ S}
        &  \small \rotatebox[origin=c]{0}{R $\rightarrow$ P}
        &  \small \rotatebox[origin=c]{0}{S $\rightarrow$ P}
        &  \small \rotatebox[origin=c]{0}{R $\rightarrow$ S}
        & \small \textbf{Avg} \\  
        \midrule
        Mean & 77.8 & 77.4 & 66.4 & 75.1 & 75.4 & 66.3 & 73.1 \\
        STD & 0.4 & 0.3 & 0.3 & 0.8 & 0.6 & 0.4 & 0.2 \\
        \bottomrule
        \end{tabular}
    }
    \label{table:multiple_run}
\end{table}
\begin{figure*}[t]
    \vspace{2mm}
    \centering
    \begin{minipage}{0.33\textwidth}
        % \label{fig:p_size}
        \centering
        \includegraphics[width=.99\linewidth]{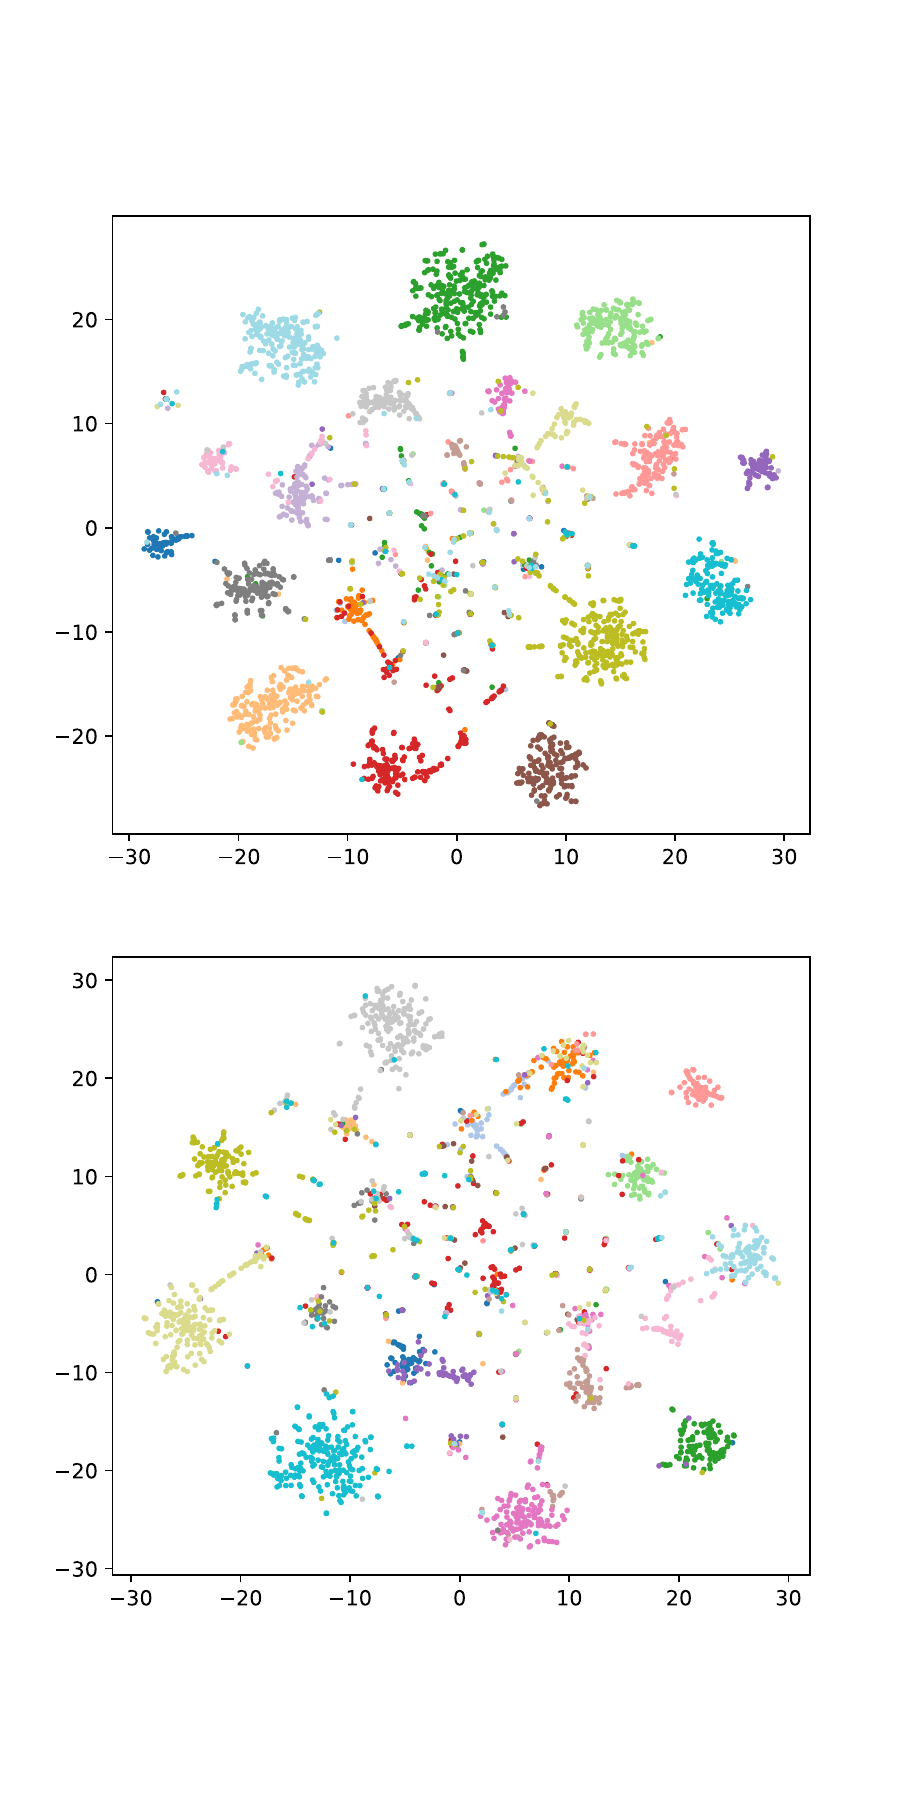}\\
        (a) MME.
    \end{minipage}
    \begin{minipage}{.33\textwidth}
        \centering
        \includegraphics[width=.99\linewidth]{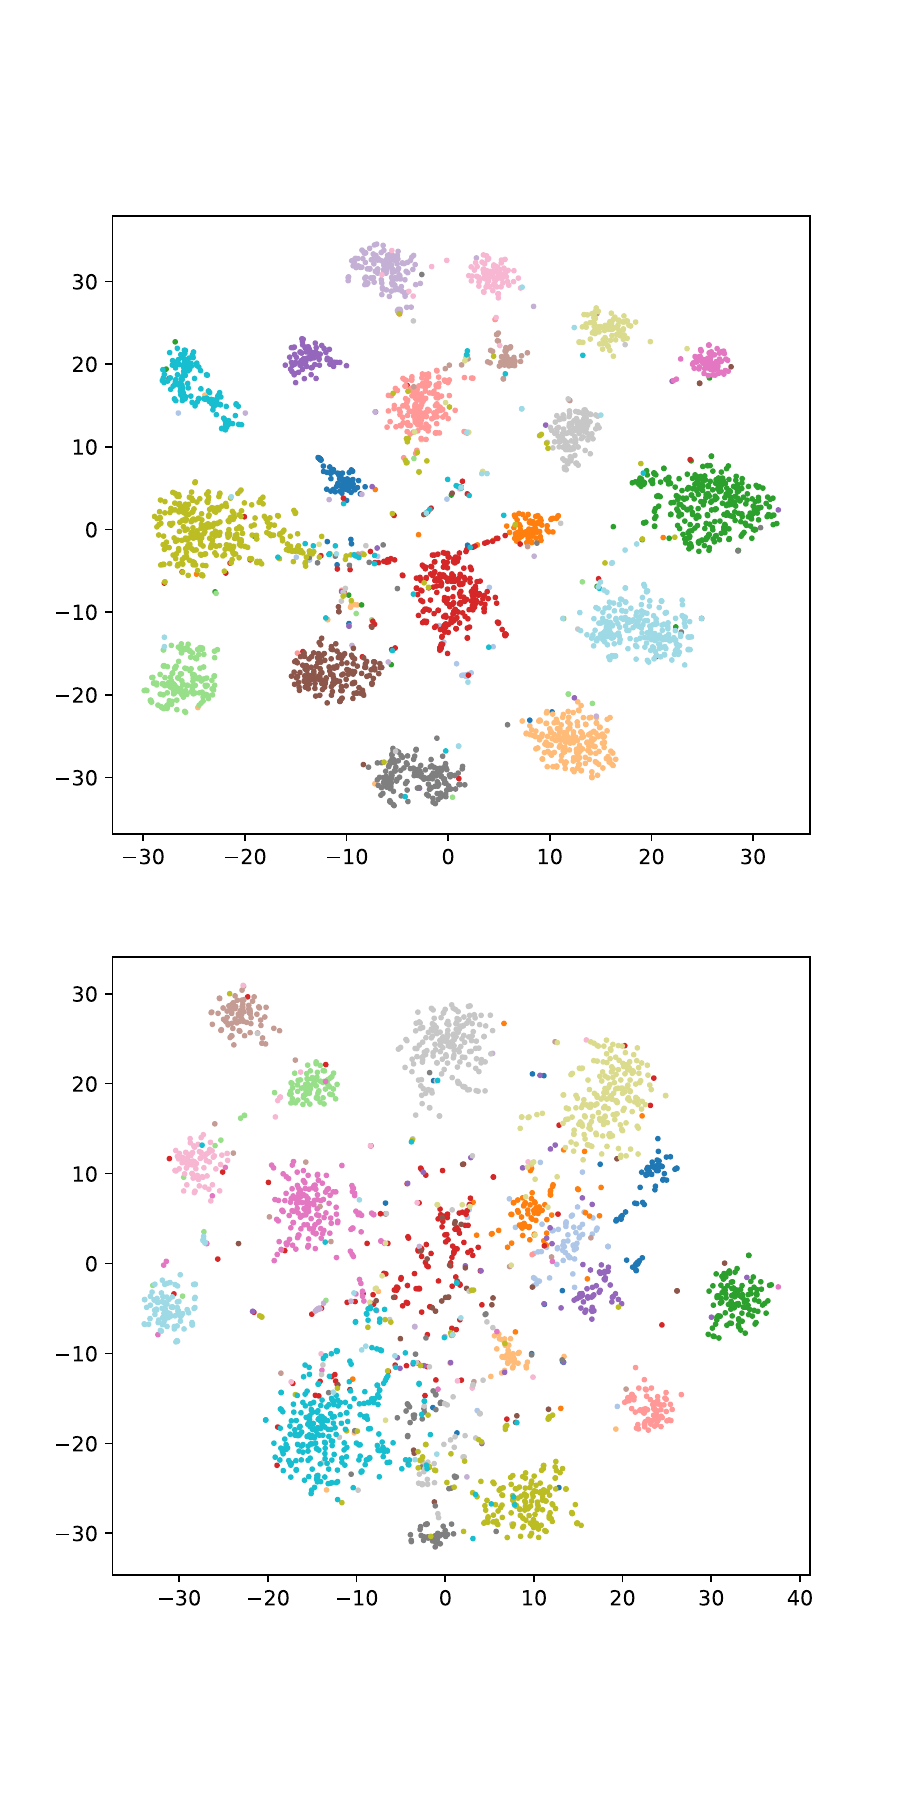}\\
        (b) FixMatch.
        % \label{fig:c_size}
        \end{minipage}%
    \begin{minipage}{.33\textwidth}
    \centering
        \includegraphics[width=.99\linewidth]{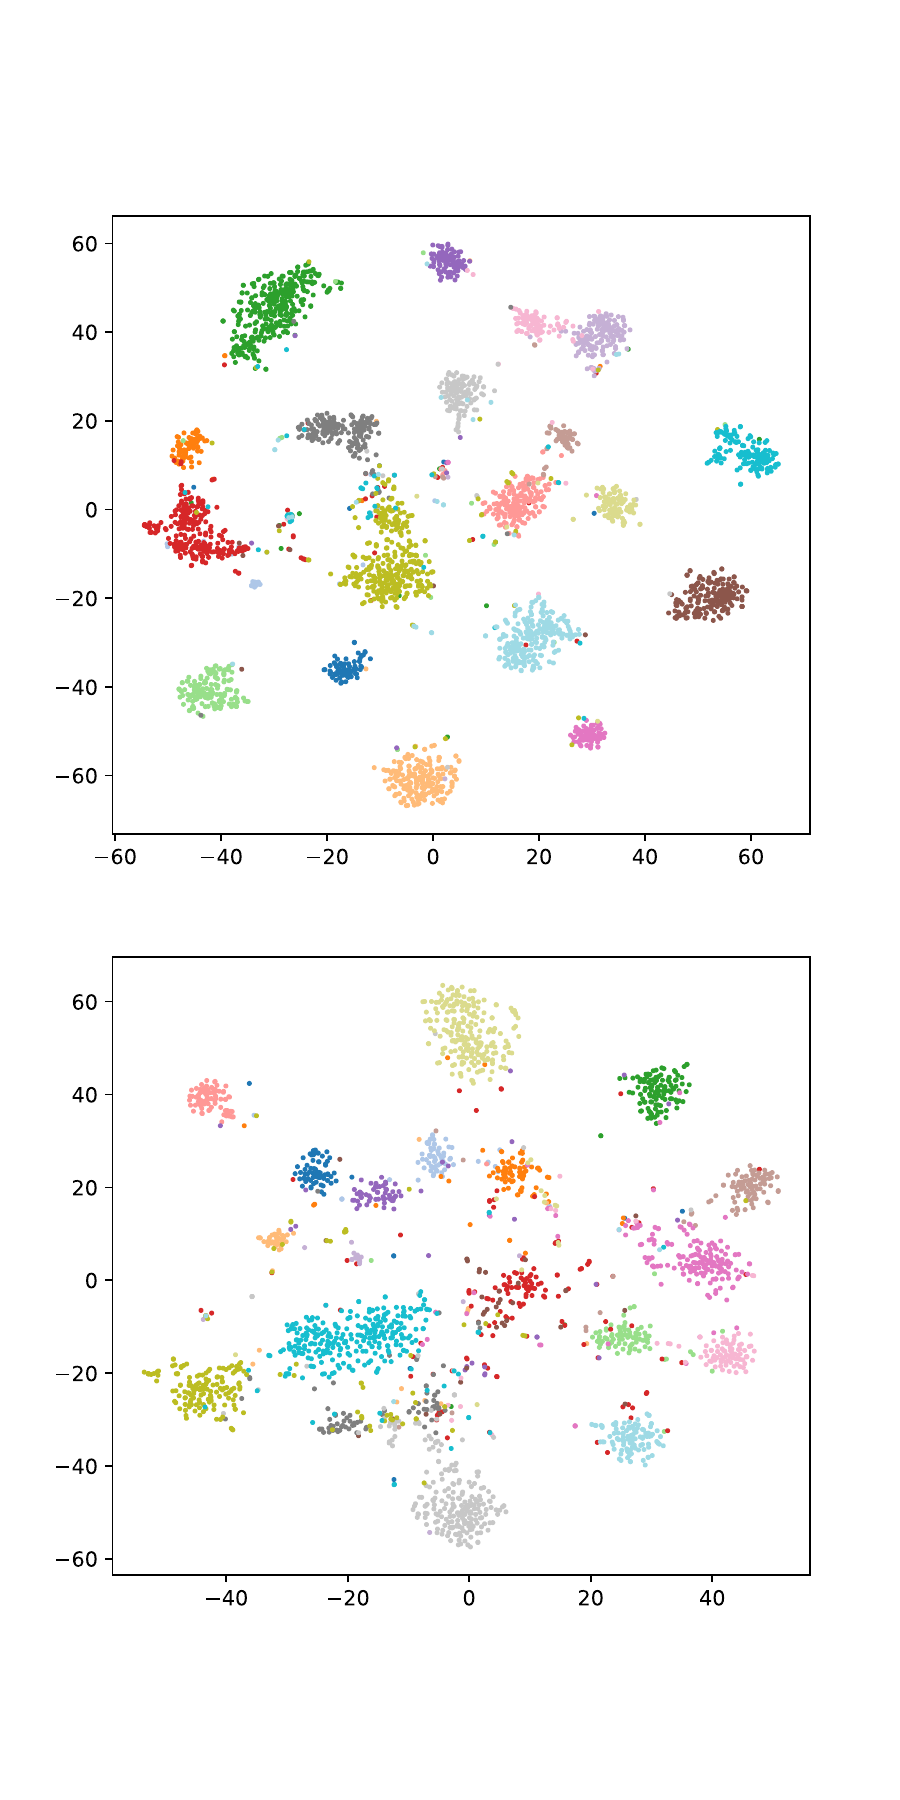}\\
        (c) CCT.
        % \label{fig:num_shot}
    \end{minipage}%
    \caption{TSNE~\cite{van2008tsne} visualization of the learned features of common~(top) and private~(bottom) sets samples respectively. We randomly sample 20 classes for both sets in task R $\rightarrow$ C on \textit{Domainnet}.}
    \label{fig:tsne}
    % \vspace{-2mm}
\end{figure*}
We investigate the performance stability of the proposed CCT in multiple runs. Table~\ref{table:multiple_run} shows the results of averaged H-score and the standard deviation of five runs on \textit{Domainnet} in the 5-shot setting. The standard deviation of the averaged H-score is very small, \ie 0.2, demonstrating the stability of our CCT.

\subsection{Feature Visualization}
In addition to the quantitative results, we also show the qualitative results of the learned features by TSNE~\cite{van2008tsne}. As Fig.~\ref{fig:tsne} shows, the features of CCT are more compact and form into well-separated clusters in both common and private sets, which verifies that our CCT learns more discriminative features.
